# Supplementary material for: Detecting and Restoring Non-Standard Hands in Stable Diffusion Generated Images
Source: arXiv:2312.04236 source file (2023-12-07)
Supplement: Supplementary file 1 [file O-z-appendix-1.tex]

\chapter{Appendix: Prompt when training IP2P}\label{chap:appendix1}

\begin{itemize}
    \item Transform the distorted hand into a regular shape
    \item Convert the abnormal hand to a normal one
    \item Change the misshapen hand into a standard form
    \item Modify the irregular hand into a typical shape
    \item Alter the twisted hand to appear normal
    \item Make the malformed hand look ordinary
    \item Adjust the deformed hand to a normal appearance
    \item Correct the unusual hand to a conventional form
    \item Revise the warped hand into a normal state
    \item Restore the irregular hand to a standard look
    \item Reshape the disfigured hand into a normal one
    \item Reform the abnormal hand into a regular shape
    \item Remodel the distorted hand to look normal
    \item Renovate the twisted hand into a standard appearance
    \item Recondition the misshapen hand into a normal state
    \item Refashion the deformed hand into a typical form
    \item Reconfigure the irregular hand to appear normal
    \item Recast the abnormal hand into a conventional shape
    \item Realign the distorted hand to a normal look
    \item Reconstruct the twisted hand into a standard form
    \item Normalize the deformed hand's appearance
    \item Rehabilitate the irregular hand to normality
    \item Refine the misshapen hand into a standard state
    \item Reorient the abnormal hand to appear normal
    \item Morph the distorted hand into a regular shape
    \item Convert the warped hand into a normal appearance
    \item Revamp the misshapen hand into a typical form
    \item Reinvent the deformed hand's look to normal
    \item Reengineer the twisted hand into a conventional shape
    \item Remake the abnormal hand into a standard form
    \item Resculpt the irregular hand into a normal look
    \item Rebuild the distorted hand to a normal state
    \item Revitalize the twisted hand into a typical shape
    \item Rework the misshapen hand to appear normal
    \item Redesign the deformed hand into a regular form
    \item Redo the abnormal hand to a standard appearance
    \item Recreate the distorted hand into a normal state
    \item Redefine the twisted hand into a typical look
    \item Reestablish the misshapen hand as normal
    \item Refurbish the irregular hand into a conventional shape
    \item Remold the deformed hand to a standard look
    \item Reawaken the abnormal hand to normality
    \item Retool the distorted hand into a regular shape
    \item Refit the twisted hand to a normal appearance
    \item Reimagine the misshapen hand into a typical form
    \item Resurrect the deformed hand into a conventional look
    \item Reenergize the irregular hand to a standard state
    \item Revise the abnormal hand to appear normal
    \item Rejuvenate the distorted hand into a regular form
    \item Reinvigorate the twisted hand to a normal state
\end{itemize}

% \begin{lstlisting}
% Transform the distorted hand into a regular shape
% Convert the abnormal hand to a normal one
% Change the misshapen hand into a standard form
% Modify the irregular hand into a typical shape
% Alter the twisted hand to appear normal
% Make the malformed hand look ordinary
% Adjust the deformed hand to a normal appearance
% Correct the unusual hand to a conventional form
% Revise the warped hand into a normal state
% Restore the irregular hand to a standard look
% Reshape the disfigured hand into a normal one
% Reform the abnormal hand into a regular shape
% Remodel the distorted hand to look normal
% Renovate the twisted hand into a standard appearance
% Recondition the misshapen hand into a normal state
% Refashion the deformed hand into a typical form
% Reconfigure the irregular hand to appear normal
% Recast the abnormal hand into a conventional shape
% Realign the distorted hand to a normal look
% Reconstruct the twisted hand into a standard form
% Normalize the deformed hand's appearance
% Rehabilitate the irregular hand to normality
% Refine the misshapen hand into a standard state
% Reorient the abnormal hand to appear normal
% Morph the distorted hand into a regular shape
% Convert the warped hand into a normal appearance
% Revamp the misshapen hand into a typical form
% Reinvent the deformed hand's look to normal
% Reengineer the twisted hand into a conventional shape
% Remake the abnormal hand into a standard form
% Resculpt the irregular hand into a normal look
% Rebuild the distorted hand to a normal state
% Revitalize the twisted hand into a typical shape
% Rework the misshapen hand to appear normal
% Redesign the deformed hand into a regular form
% Redo the abnormal hand to a standard appearance
% Recreate the distorted hand into a normal state
% Redefine the twisted hand into a typical look
% Reestablish the misshapen hand as normal
% Refurbish the irregular hand into a conventional shape
% Remold the deformed hand to a standard look
% Reawaken the abnormal hand to normality
% Retool the distorted hand into a regular shape
% Refit the twisted hand to a normal appearance
% Reimagine the misshapen hand into a typical form
% Resurrect the deformed hand into a conventional look
% Reenergize the irregular hand to a standard state
% Revise the abnormal hand to appear normal
% Rejuvenate the distorted hand into a regular form
% Reinvigorate the twisted hand to a normal state
% \end{lstlisting}
